# Supplementary material for: Dynamic Programming in Probability Spaces via Optimal Transport
Source: arXiv:2302.13550 source file (2024-04-08)
Supplement: Supplementary file 1 [file A_Preliminaries.tex]

\section{Preliminaries of Measure Theory and Optimal Transport}
In this section we recall two complementary results in Measure Theory.

\begin{theorem}[Disintegration theorem {\cite[Theorem 5.3.1]{Ambrosio2008}}]\label{theorem:disintegration}
Let $\mu \in \spaceProbabilityBorelMeasures{X}$ and let $\pi: X \to Y$ be a Borel map. Define $\nu = \pushforward{\pi}{\mu} \in \spaceProbabilityBorelMeasures{Y}$. There exists $\nu\ae{}$ uniquely determined $\{\mu_y\}_{y \in Y} \subset \spaceProbabilityBorelMeasures{X}$ such that
$
\mu_y(X \setminus \pi^{-1}(y)) = 0\text{ for }\nu\ae{}\,y \in Y
$,
$
\int_X \phi(x)\d\mu(x) = \int_Y\int_{\pi^{-1}(y)}\phi(x)\d\mu_y(x)\d\nu(y).
$
, and the map $y \mapsto \mu_y$ is Borel.
\end{theorem}

\begin{theorem}[{\cite[Gluing lemma]{Villani2007}}]\label{theorem:gluinglemma}
Consider $\mu_i \in \spaceProbabilityBorelMeasures{X_i}$ for Polish spaces $X_i$, $i \in \{1,2,3\}$. If $\mu_{12} \in \setPlans{\mu_1}{\mu_2}$ and $\mu_{23} \in \setPlans{\mu_2}{\mu_3}$, then one can construct a Borel probability measure $\mu_{123} \in \spaceProbabilityBorelMeasures{X_1 \times X_2 \times X_3}$ such that 
$
\pushforward{\pi_{12}}{\mu_{123}} = \mu_{12}
$
and
$
\pushforward{\pi_{23}}{\mu_{123}} = \mu_{23}.
$
\end{theorem}

\begin{comment}
\begin{theorem}[{\cite[Theorem 5.10, Kantorovich Duality]{Villani2007}}]\label{theorem:kantorovichduality}
For $X,Y$ polish spaces, $\mu \in \spaceProbabilityBorelMeasures{X}$, $\nu \in \spaceProbabilityBorelMeasures{Y}$, and $c \in \lsc{X\times Y}{[0,\infty]}$, there is duality:
\begin{multline*}
\min_{\plan{\gamma} \in \setPlans{\mu}{\nu}} \int_{X \times Y} c(x,y) \d\plan{\gamma}(x,y)\\
=\sup\left\{ \int_X\phi(x)\d\mu(x) - \int_Y\psi(y)\d\nu(y) \st \phi \in \Cb{X}, \psi \in \Cb{Y}, \phi - \psi \preceq c\right\}.
\end{multline*}
\end{theorem}

The statement of \cite[Theorem 5.10]{Villani2007} is comprehensive of different declinations; for instance, the $\sup$ can be attained with some extra assumptions. However, in this work the statement provided suffices, and we simplify the notation as:
\begin{multline*}
\sup\biggl\{ \int_X\phi(x)\d\mu(x) - \int_Y\psi(y)\d\nu(y) \st \phi \in \Cb{X}, \psi \in \Cb{Y}, \phi - \psi \preceq c\biggr\}
\\
\eqqcolon \sup_{\phi,\psi} \int_X\phi(x)\d\mu(x) - \int_Y\psi(y)\d\nu(y).
\end{multline*}
\end{comment}
